# Supplementary material for: Multiscale Feature Learning Using Co-Tuplet Loss for Offline Handwritten Signature Verification
Source: arXiv:2308.00428 source file (2025-08-30)
Supplement: Supplementary file 1 [file supplemental_material.pdf]

# Multiscale Global and Regional Feature Learning Using Co-Tuplet Loss for Offline Handwritten Signature Verification

## Supplemental Material

### I. OVERVIEW

In this supplemental material, we first present the CNN backbone of the proposed MGRNet. Then we provide the gradient computation of our proposed co-tuplet loss. After that, we describe the collection process of our newly created HanSig dataset, followed by displaying examples before and after data preprocessing. Finally, we evaluate the validity of the selected operations and show that our backbone and MGRNet are parameter-efficient compared to several deep networks.

### II. LAYERS OF OUR CNN BACKBONE

The layers of our CNN backbone used to build the branches and modules of the MGRNet are summarized in TABLE I.

TABLE I

SUMMARY OF OUR CNN BACKBONE. EXCEPT FOR THE FULLY CONNECTED LAYER, ALL SIZES ARE DESCRIBED IN  $DEPTH \times HEIGHT \times WIDTH$

| Layer                        | Size                      | Stride & Padding    |
|------------------------------|---------------------------|---------------------|
| Input                        | $1 \times 150 \times 220$ |                     |
| Convolution (Conv1)          | $96 \times 11 \times 11$  | Stride = 1, pad = 0 |
| Pooling                      | $96 \times 3 \times 3$    | Stride = 2          |
| Convolution (Conv2)          | $256 \times 5 \times 5$   | Stride = 1, pad = 2 |
| Pooling                      | $256 \times 3 \times 3$   | Stride = 2          |
| Convolution (Conv3)          | $384 \times 3 \times 3$   | Stride = 1, pad = 1 |
| Convolution (Conv4)          | $384 \times 3 \times 3$   | Stride = 1, pad = 1 |
| Convolution (Conv5)          | $256 \times 3 \times 3$   | Stride = 1, pad = 1 |
| Pooling                      | $256 \times 3 \times 3$   | Stride = 2          |
| Global average pooling (GAP) | $256 \times 1 \times 1$   |                     |
| Fully connected (FC)         | 1,024                     |                     |

### III. GRADIENT COMPUTATION OF CO-TUPLET LOSS

We can obtain the gradient of the proposed co-tuplet loss with respect to the model parameters  $\theta$ . The gradient computation is as follows:

$$\begin{aligned} \frac{\partial \mathcal{L}_{ct}}{\partial \theta} &= \frac{1}{q} \left[ \sum_{i \in \mathcal{S}(\mathcal{P})} \exp(d_i^+ - d_h^-) \frac{\partial (d_i^+ - d_h^-)}{\partial \theta} \right. \\ &\quad \left. + \sum_{j \in \mathcal{S}(\mathcal{N})} \exp(d_h^+ - d_j^-) \frac{\partial (d_h^+ - d_j^-)}{\partial \theta} \right] \\ &\equiv \frac{1}{q} \left[ \sum_{i \in \mathcal{S}(\mathcal{P})} w_{1,i} \frac{\partial (d_i^+ - d_h^-)}{\partial \theta} \right. \\ &\quad \left. + \sum_{j \in \mathcal{S}(\mathcal{N})} w_{2,j} \frac{\partial (d_h^+ - d_j^-)}{\partial \theta} \right], \end{aligned} \quad (1)$$

where

$$q = 1 + \sum_{i \in \mathcal{S}(\mathcal{P})} \exp(d_i^+ - d_h^-) + \sum_{j \in \mathcal{S}(\mathcal{N})} \exp(d_h^+ - d_j^-), \quad (2)$$

and  $w_{1,i}$  and  $w_{2,j}$  denote the weights of the pulling and pushing parts, respectively. As observed from the above gradient, both  $w_{1,i}$  and  $w_{2,j}$  are exponentially up-weighted with hard examples and exponentially down-weighted with easy ones.

In comparison to typical metric learning losses, our co-tuplet loss offers the advantage of emphasizing informative examples over uninformative ones by assigning unequal weights to examples based on the distance difference in  $d_i^+ - d_h^-$  and  $d_h^+ - d_j^-$ . Since skilled-forged signatures often closely resemble genuine signatures for each writer, this weighting scheme promotes the learning of more discriminative features for handwritten signature verification. Furthermore, our proposed loss function takes into account moderate examples (i.e., the examples of normal cases) for distance learning. As a result, it avoids overweighting extremely hard examples, leading to a more stable optimization process.

### IV. DATA COLLECTION PROCESS OF HANSIG

Due to the scarcity of large-scale public offline Chinese signature datasets, we construct the HanSig dataset to be made publicly available and to facilitate the development of signature verification systems. To begin, we collected 554,723 names from the Joint College Entrance Exam admissions lists between 1996 and 2002. These names were further divided into first names and last names, and we filtered out the first and last names that appeared less than two times. Next, we generated 885 candidate names based on the frequency distributions of the first and last names to match the name distribution in the real world. By generating candidate names,

we took precautions to avoid potential legal concerns related to personal information.

To create genuine signatures, we assigned the previously generated candidate names to 238 writers. Each writer was allocated either three or six candidate names and asked to sign each name 20 times. To introduce more variations in the genuine signatures, we requested each writer to sign each candidate name in three different styles: neat, normal, and stylish. The genuine signatures were subsequently passed on to another writer, referred to as the forger, to create forged signatures. Because this study aims to distinguish between genuine signatures and skilled forgeries, we requested the forgers to practice and skillfully imitate the genuine signatures to create forged signatures. Overall, the HanSig dataset consists of a total of 35,400 signature samples (17,700 genuine signatures and an equal number of skilled forgeries).

## V. EXAMPLES OF DATA PREPROCESSING

Fig. 1 displays examples of CEDAR before and after the data preprocessing steps (excluding the last step of normalization of pixel values). This figure shows that removing noise in image backgrounds is critical to datasets (e.g., CEDAR) that have distinct backgrounds in genuine and forged signature images.

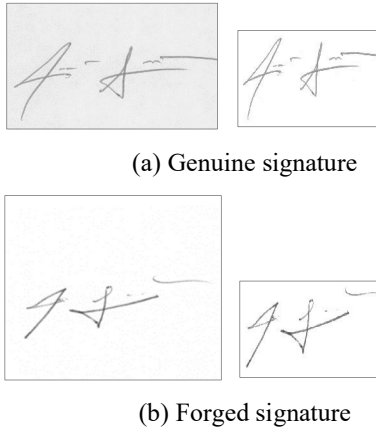

**Fig. 1.** Examples of CEDAR before and after preprocessing. The left images of (a) and (b) are original signature images, and the right images are preprocessed results.

## VI. ABLATION STUDY - VALIDITY OF SELECTED OPERATIONS

To evaluate the validity of the selected operations for multilevel feature fusion and model training, we compare the signature verification performances on CEDAR using different operations while maintaining the same experimental settings. The results of this comparison are presented in TABLE II. Regarding multilevel feature fusion, the original “multiplication” is compared with the conventional “concatenation” as the fusion strategy for combining low-level and high-level features. The results demonstrate that using “multiplication” leads to a significant improvement in EER by 4.32 percentage points compared to using “concatenation.”

This indicates the superiority of the multiplicative operation, which promotes interaction between low-level and high-level features during training and contributes to enhanced performance.

For model training, the original approach involves training each set of global and regional features with individual co-tuplet losses, which enforces the model to learn specific global and regional information. In contrast, an alternative approach is employed where the features are concatenated and trained with only one loss during the learning process. The results in TABLE II reveal that training “with individual losses” outperforms training “with only one loss” by 5.04 percentage points. This suggests that training with individual losses allows the model to learn more discriminative representations and leads to improved signature verification performance.

**TABLE II**  
PERFORMANCE COMPARISON BETWEEN DIFFERENT OPERATIONS ON CEDAR (EER IN %)

|                           | Operation                     | EER         |
|---------------------------|-------------------------------|-------------|
| Multilevel feature fusion | Concatenation                 | 7.83        |
|                           | Multiplication (Ours)         | <b>3.51</b> |
| Model training            | With only one loss            | 8.55        |
|                           | With individual losses (Ours) | <b>3.51</b> |

## VII. COMPARISON OF THE NUMBER OF PARAMETERS

The backbone of our handwritten signature verification system consists of only five convolutional layers and one FC layer, which is more parameter-efficient than the very deep networks, such as VGGNet [1], ResNet [2], and DenseNet [3], as shown in TABLE III. This makes our MGRNet more lightweight than existing signature verification systems based on these deep networks [4]–[7]. Our MGRNet that requires less computation complexity can be easily trained on small signature datasets to achieve competitive performance, even without pretraining on large datasets.

**TABLE III**  
COMPARISON OF THE NUMBER OF LEARNABLE PARAMETERS. ALL METHODS ARE SET TO HAVE THE SAME OUTPUT DIMENSION OF 1,024

| Method           | #Params      |
|------------------|--------------|
| CNN Backbone     |              |
| VGG-16 [1]       | 117.48M      |
| ResNet-18 [2]    | 11.69M       |
| DenseNet-121 [3] | 8.00M        |
| Ours             | <b>3.99M</b> |
| MGRNet (Ours)    | <b>7.96M</b> |

## REFERENCES

- [1] K. Simonyan and A. Zisserman, “Very deep convolutional networks for large-scale image recognition,” in *Proc. Int. Conf. Learn. Represent. (ICLR)*, San Diego, CA, USA, 2015.
- [2] K. He, X. Zhang, S. Ren, and J. Sun, “Deep residual learning for image recognition,” in *Proc. IEEE Conf. Comput. Vis. Pattern Recognit. (CVPR)*, Las Vegas, NV, USA, 2016, pp. 770–778.
- [3] G. Huang, Z. Liu, L. Van Der Maaten, and K. Q. Weinberger, “Densely connected convolutional networks,” in *Proc. IEEE Conf. Comput. Vis. Pattern Recognit. (CVPR)*, Honolulu, HI, USA, 2017, pp. 2261–2269.
- [4] L. Liu, L. Huang, F. Yin, and Y. Chen, “Offline signature verification using a region based deep metric learning network,” *Pattern Recognit.*, vol. 118, p. 108009, 2021.
- [5] P. Maergner, V. Pondenkandath, M. Alberti, M. Liwicki, K. Riesen, R. Ingold, and A. Fischer, “Combining graph edit distance and triplet networks for offline signature verification,” *Pattern Recognit. Lett.*, vol. 125, pp. 527–533, 2019.
- [6] S. Bonde, P. Narwade, and R. Sawant, “Offline signature verification using convolutional neural network,” in *Proc. IEEE Int. Conf. Signal Process. Comput.*, Noida, India, 2020, pp. 119–127.
- [7] S. Chattopadhyay, S. Manna, S. Bhattacharya, and U. Pal, “SURDS: Self-supervised attention-guided reconstruction and dual triplet loss for writer independent offline signature verification,” in *Proc. 26th Int. Conf. Pattern Recognit.*, Montreal, QC, Canada, 2022, pp. 1600–1606.
